# Supplementary material for: Modulo Sampling: Performance Guarantees in The Presence of Quantization
Source: arXiv:2501.01506 source file (2025-08-30)
Supplement: Supplementary file 4 [file appendix_D.tex]

\documentclass[../main.tex]{subfiles}

\begin{document}
From Theorem \ref{theorem:quant_noise}, $z[n] - \hat{z}[n] = 0$ if $b > 3$ and $\mathrm{OF} > 3$. The normalized MSE of recovering the $i$-th component becomes
    \begin{align}
        \frac{\mathbb{E}[(\alpha_if_i[n] - \hat{f}_i[n])^2]}{\mathbb{E}[(\alpha_if_i[n])^2]} =& \frac{1}{\alpha_i^2}\mathbb{E}[(\mathrm{BPF}_{i}\{\epsilon[n]\})^2]\nonumber\\
        = & \frac{\rho}{\alpha_i^2}\cdot \frac{\omega_i}{\omega_m}\cdot\frac{2\lambda'^2}{(2^{b}-2)^2}.
    \end{align}
    Setting $\lambda'$ to be the RHS of \eqref{eq:lambda_requirement} and replacing $\|f(t)\|_{\infty}$ by its upper bound $\sqrt{\frac{\omega_m(\alpha_1^2+\alpha_2^2)}{\pi}}$ complete the proof.
\end{document}
